# Supplementary material for: Sentry: Authenticating Machine Learning Artifacts on the Fly
Source: arXiv:2510.00554 source file (2025-10-01)
Supplement: Supplementary file 1 [file appendix.tex]

%%%%%%%%%%%%%%%%%%%%%%%%%%%%%%%%%%%%%%%%%%%%%%%%%%%%
% When adding this appendix to your paper, 
% please remove the part above
%%%%%%%%%%%%%%%%%%%%%%%%%%%%%%%%%%%%%%%%%%%%%%%%%%%%

\appendix
\section{Artifact Appendix}

%%%%%%%%%%%%%%%%%%%%%%%%%%%%%%%%%%%%%%%%%%%%%%%%%%%%
% See the Artifact Appendix guidelines page on the USENIX
% Security website to compile the appendix. Please preserve
% the provided Artifact Appendix template as much as
% possible (e.g., keep the original (sub)section names
% and order). 
%
% See also examples of past reproduced papers with a similar Artifact Appendix at: https://cknowledge.io/?q=%22reproduced-papers%22+AND+lib+AND+%28secur*+OR+harden*+OR+mitigat*+OR+defen*+OR+attack*+OR+bug*+OR+vulnerab*%29
%%%%%%%%%%%%%%%%%%%%%%%%%%%%%%%%%%%%%%%%%%%%%%%%%%%%

%%%%%%%%%%%%%%%%%%%%%%%%%%%%%%%%%%%%%%%%%%%%%%%%%%%%%%%%%%%%%%%%%%%%%
\subsection{Abstract}

{\em The artifact has a Python code base and CUDA kernels. Calls between both are done using Cython and CUDA Python. Minimal hardware requirements include an Nvidia GPU that runs CUDA>=12.6 and Python packages listed in requirements.txt. The README.md details steps to replicate workflow and obtain key results. The code has print statements to show runtime and status updates after every important step is completed. We also support docker for ease of running the artifact.

\subsection{Artifact check-list (meta-information)}

{\small
\begin{itemize}
  \item {\bf Algorithm: SHA256, BLAKE2, SHA3, Lattice Hashing, Merkle Tree, ECDSA}
  \item {\bf Program: Sentry, Docker, PyTorch}
  \item {\bf Compilation: NVRTC, NVCC }
  \item {\bf Model: ResNet121, Bert, VGG19, GPT2, GPT2-XL}
  \item {\bf Data set: CIFAR10, hellaswag}
  \item {\bf Run-time environment: Docker or Python venv}
  \item {\bf Hardware: V100, A30, A100, RTX A6000}
  \item {\bf Metrics: runtime, memory}
  \item {\bf Output: Signatures for each model and dataset curator}
  \item {\bf How much disk space required?: 16 GB}
  \item {\bf How much time is needed to prepare workflow?: if Docker, 5 minutes}
  \item {\bf How much time is needed to complete experiments?: < 1 minute}
  \item {\bf Publicly available?: https://github.com/Andrew-Gan/sentry}
  \item {\bf Workflow frameworks used?: Sigstore, DALI}
  \item {\bf Archived?: 10.5281/zenodo.16905016}
\end{itemize}

%%%%%%%%%%%%%%%%%%%%%%%%%%%%%%%%%%%%%%%%%%%%%%%%%%%%%%%%%%%%%%%%%%%%%
\subsection{Description}

\subsubsection{How to access}
Visit https://github.com/Andrew-Gan/sentry or https://zenodo.org/records/16953160.

\subsubsection{Hardware dependencies}
Any Nvidia GPU that runs CUDA 12.6 or above. To run with GPUDirect Storage, make sure the GPU supports GPUDirect Storage. To disable using GDS, the GDS argument to $get\_image\_dataloader$ in $agent\_trainer.py and agent\_inferencer.py$ should be set to false. There is no specific CPU requirement.

\subsubsection{Software dependencies}

A GPU driver and CUDA toolkit compatible with the available Nvidia GPU should be installed.\\
If running with Docker, install docker engine, docker compose and the necessary prerequisites to use docker with GPU support. If without Docker, Python>=3.10, openssl and nvcc are needed.

\subsubsection{Data sets}

The dataset generation script fetches and generates numpy array version of CIFAR10 and hellaswag. Numpy array formatting is needed for the DALI dataloader to load datasets through GPUDirect Storage. Even if GDS is disabled, datasets will still be loaded in numpy array format.

\subsubsection{Models}

The code base automatically fetches specified models from Huggingface and loads them into GPU memory. Currently supported models are ResNet121, BERT, VGG19, GPT2 and GPT2-XL, but more can be added by finding, from the desired model's Huggingface page, the function calls needed to load them into the PyTorch framework.

\subsubsection{Security, privacy, and ethical concerns}

This artifact makes use of remote artifacts for building the machine learning supply chain. However, the datasets and models are publicly available and pretrained, so no privacy concerns are known.

%%%%%%%%%%%%%%%%%%%%%%%%%%%%%%%%%%%%%%%%%%%%%%%%%%%%%%%%%%%%%%%%%%%%%
\subsection{Installation}

Installation steps are detailed in the artifact's README.md.\\
For quick docker setup, the following commands will suffice.
\begin{lstlisting}
mkdir -p ./signatures
docker compose up --build sentry_dataset
docker compose up --build sentry_trainer
docker compose up --build sentry_inferencer
\end{lstlisting}

%%%%%%%%%%%%%%%%%%%%%%%%%%%%%%%%%%%%%%%%%%%%%%%%%%%%%%%%%%%%%%%%%%%%%
\subsection{Experiment workflow}

First, a dataset curation Python script fetches and formats raw data before storing it. Next, the model trainer Python script fetches the model and datasets to train. The model trainer then signs the trained models and datasets (we assume trainer and dataset curator are same but that can be modified) and writes the signatures to a file. Finally, the model inferencer Python script fetches the pretrained model and datasets for inference. It opens the signatures and verifies model and dataset authenticity.

%%%%%%%%%%%%%%%%%%%%%%%%%%%%%%%%%%%%%%%%%%%%%%%%%%%%%%%%%%%%%%%%%%%%%
\subsection{Evaluation and expected results}

In the code base, the default configuration for model hashing produces the best runtime results, which is SHA256 with Merkle inplace mode. As stated in the results section, the hashing runtime decreased from 165.6 ms to 5.53 ms on an RTX A6000. Our code base should print out a runtime message indicating a similar runtime. These configurations can be changed to obtain other key results as detailed in the next subsection.

%%%%%%%%%%%%%%%%%%%%%%%%%%%%%%%%%%%%%%%%%%%%%%%%%%%%%%%%%%%%%%%%%%%%%
\subsection{Experiment customization}

By modifying the inputs in $agent\_trainer.py$ and $agent\_inferencer.py$, one can obtain the key results for different ML models, datasets, hashing algorithms and topologies. To change the way datasets are generated, such as number of unique dataset curators in a dataset pool, modify the CMD line in the $docker-compose.yml$.

%%%%%%%%%%%%%%%%%%%%%%%%%%%%%%%%%%%%%%%%%%%%%%%%%%%%%%%%%%%%%%%%%%%%%
\subsection{Notes}

Sentry incorporated an older version of Sigstore/model-transparency in December 2024-January 2025 and can be updated as future work.

%%%%%%%%%%%%%%%%%%%%%%%%%%%%%%%%%%%%%%%%%%%%%%%%%%%%%%%%%%%%%%%%%%%%%
\subsection{Version}
%%%%%%%%%%%%%%%%%%%%
% Obligatory.
% Do not change/remove.
%%%%%%%%%%%%%%%%%%%%
Based on the LaTeX template for Artifact Evaluation V20220119.
